# Supplementary material for: Strong, Temperature-Dependent Spin-Orbit Torques in Heavy Fermion YbAl$_3$
Source: arXiv:2004.03678 ancillary file (2022-01-31)
Supplement: Supplementary file 2 [file SI_Strong__Temperature_Dependent_Spin_Torques_in_Heavy_Fermion_YbAl__3.pdf]

# Strong, Temperature-Dependent Spin-Orbit Torques in Heavy Fermion YbAl<sub>3</sub>

Neal D. Reynolds,<sup>1,\*</sup> Shouvik Chatterjee,<sup>1,\*</sup> Gregory M. Stiehl,<sup>1</sup> Joseph A. Mittelstaedt,<sup>1</sup> Saba Karimeddiny,<sup>1</sup> Alexander J. Buser,<sup>1</sup> Darrell G. Schlom,<sup>2,3</sup> Kyle M. Shen,<sup>1,3</sup> and Daniel C. Ralph<sup>1,3</sup>

<sup>1</sup>*Department of Physics, Cornell University, Ithaca, NY 14853, USA*

<sup>2</sup>*Department of Materials Science and Engineering, Cornell University, Ithaca, NY 14853, USA*

<sup>3</sup>*Kavli Institute at Cornell, Cornell University, Ithaca, NY 14853, USA*

(Dated: April 6, 2020)

## SUPPLEMENTARY INFORMATION

### A. Resistivity determination for the layers in the LuAl<sub>3</sub>/YbAl<sub>3</sub>/Fe/AlO<sub>x</sub> stack

We grew a series of heterostructures with different thicknesses for the YbAl<sub>3</sub> and Fe layers: Al 1.8 nm/LuAl<sub>3</sub> 5 nm/YbAl<sub>3</sub>  $x$  nm/Fe 6 nm/Al 3 nm ( $x = 6.7, 15, 18$ ) and Al 1.8 nm/LuAl<sub>3</sub> 5 nm/YbAl<sub>3</sub> 10 nm/Fe  $y$  nm/Al 3 nm ( $y = 3, 6, 9, 12$ ). In the heterostructures the epitaxial orientation relationship among Fe and YbAl<sub>3</sub>/LuAl<sub>3</sub> with respect to MgO is (001)[110]Fe||[(001)[100]YbAl<sub>3</sub>/LuAl<sub>3</sub>][(001)[100]MgO (Fig. S1). We assume that the top Al layer oxidizes completely upon exposure to air and thus does not contribute to the resistance of the stacks. Hall bars with length  $\times$  width dimensions of  $560 \mu\text{m} \times 110 \mu\text{m}$ ,  $240 \mu\text{m} \times 40 \mu\text{m}$ , and  $120 \mu\text{m} \times 20 \mu\text{m}$  were fabricated on the same die as the magneto optical Kerr effect (MOKE) devices and spin torque ferromagnetic resonance (ST-FMR) devices. For each film, the temperature-dependent resistivity was measured using a Hall-bar device in a Quantum Design physical properties measurement system (PPMS). We find excellent agreement between sheet resistances of the Hall bars on the same die as a function of temperature. We extract the resistivities  $\rho_{\text{YbAl}_3}$  and  $\rho_{\text{Fe}}$  from the slope of the linear regression of the sheet resistance vs.  $1/x$  or  $1/y$ , respectively. We determine  $\rho_{\text{LuAl}_3+\text{Al}}$  from the intercept of the sheet resistance vs.  $1/x$  (the YbAl<sub>3</sub> thickness series) after subtracting out the contribution due to the Fe layer using  $\rho_{\text{Fe}}$  determined from the thickness series of Fe. The resulting  $\rho$  vs.  $T$  for each layer is shown in Fig. 1a of the main text.  $\rho_{\text{YbAl}_3}$  and  $\rho_{\text{LuAl}_3+\text{Al}}$  are consistent with our previous work<sup>1</sup> and  $\rho_{\text{Fe}}$  is consistent with earlier reports as well<sup>2</sup>.

### B. Magnetic characterization of the Fe layer

As discussed in the Methods section of the main text, we perform vibrating sample magnetometry (VSM) using a Quantum Design PPMS to extract the sample saturation magnetization,  $M_s$ , for both the Fe layer in the YbAl<sub>3</sub>/Fe heterostructure (i.e. MgO (001)/Al 1.8 nm/LuAl<sub>3</sub> 5 nm/YbAl<sub>3</sub> 15 nm/Fe 6 nm/oxidized Al) and the Fe layer in the LuAl<sub>3</sub>-only control heterostructure (i.e. MgO (001)/Al 1.8 nm/LuAl<sub>3</sub> 15 nm/Fe 6 nm/oxidized Al), yielding the  $M_s$  vs.  $T$  dependence shown in Fig. S2a and d, respectively. The temperature dependence of the magnetization in the YbAl<sub>3</sub>/Fe structure appears qualitatively to follow the YbAl<sub>3</sub> susceptibility vs.  $T$  (see ref.<sup>3</sup>) in reverse, *i.e.*  $M_s$  decreases as  $\chi_{\text{YbAl}_3}$  increases, suggesting a proximity effect in which a small induced moment in YbAl<sub>3</sub> is antiparallel to that in the Fe layer. In both the YbAl<sub>3</sub> stack and the LuAl<sub>3</sub> only stack, the Fe layer saturation magnetization is slightly smaller than the  $1.71 \times 10^6$  A/m saturation magnetization for bulk, crystalline Fe<sup>4</sup>.

The in-plane angular dependence of the resonant field reveals a moderate bi-axial magnetocrystalline anisotropy field with easy axes along the substrate diagonals, corresponding to the Fe [100] directions (and parallel to the YbAl<sub>3</sub> [110] directions, see Fig. S1). No additional uniaxial anisotropy was observed, which is expected because the substrates were continuously rotated during the deposition process. A representative trace at 40 K is shown in Fig. S2b) with a fit to

$$B_{\text{res}} = \frac{1}{8} \left( \sqrt{64 \frac{\omega^2}{\gamma^2} + 9H_a^2 + 24H_a M_{\text{eff}} + 16M_{\text{eff}}^2 + 9H_a^2 \cos^2(4\phi) + (18H_a^2 + 24H_a M_{\text{eff}}) \cos(4\phi)} \right. \\ \left. + 5H_a \cos(4\phi) - 3H_a - 4M_{\text{eff}} \right) \quad (\text{S1})$$

---

\* equal contribution

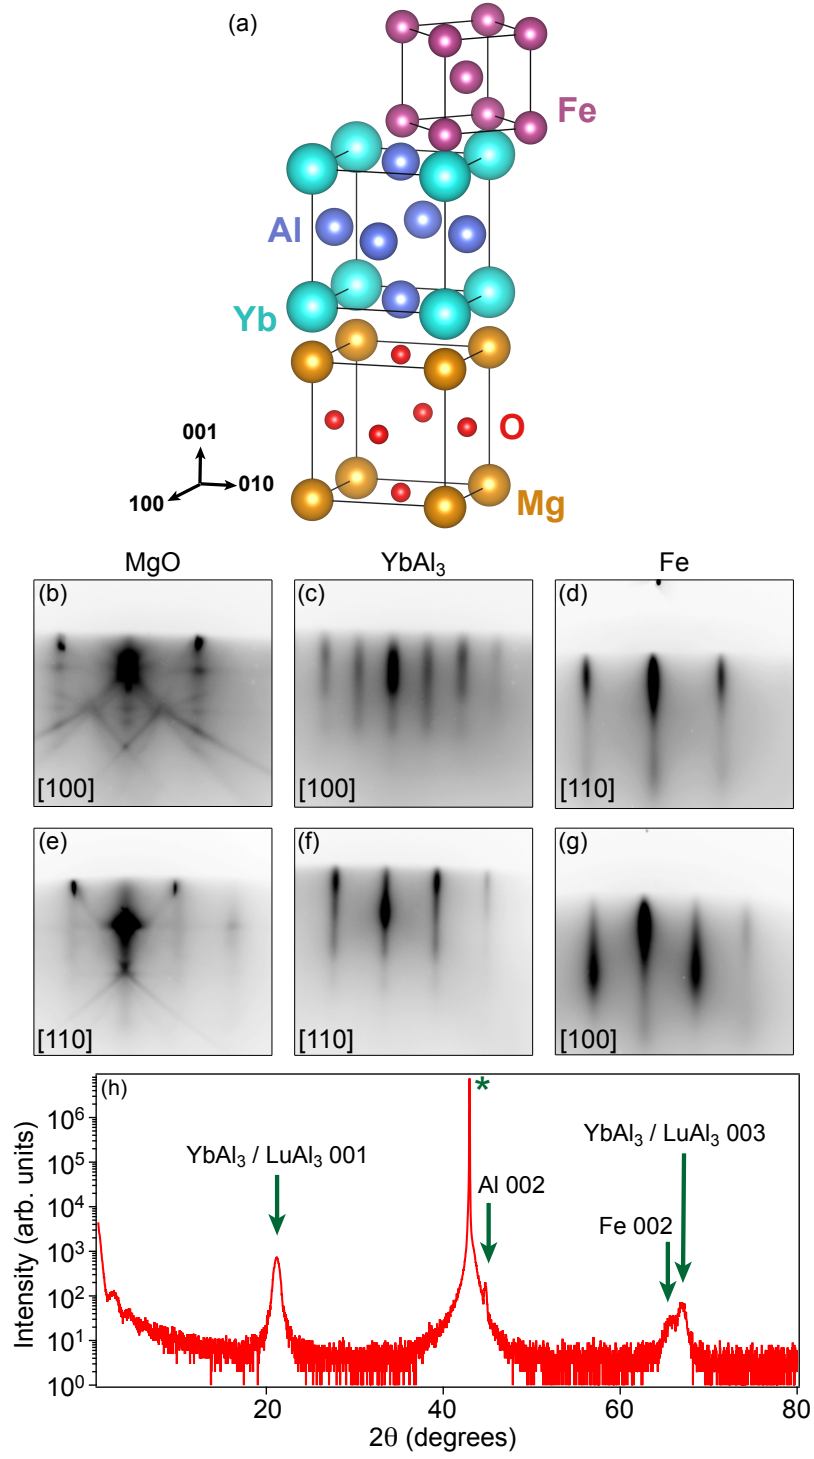

FIG. S1. (a) An atomic model illustrating the orientation relationship between MgO, YbAl<sub>3</sub> and Fe layers in the heterostructure used for ST-FMR and MOKE measurements. (b-g) Reflection high-energy electron diffraction (RHEED) images at different stages of the growth process of a heterostructure similar to the one used for ST-FMR and MOKE measurements. Images taken along the [100] azimuth of the MgO substrate (b) prior to the start of the growth process, (c) after YbAl<sub>3</sub> deposition, and (d) after Fe deposition. (e-g) Corresponding RHEED images along the [110] azimuth of the MgO substrate. (h) Out-of-plane  $\theta$  -  $2\theta$  x-ray diffraction scan (XRD) of the heterostructure taken with Cu K $\alpha_1$  radiation. The substrate peak is indicated by an asterisk. The RHEED images along with the XRD scan establish the epitaxial relationship between MgO, YbAl<sub>3</sub> and Fe layers in the heterostructure.

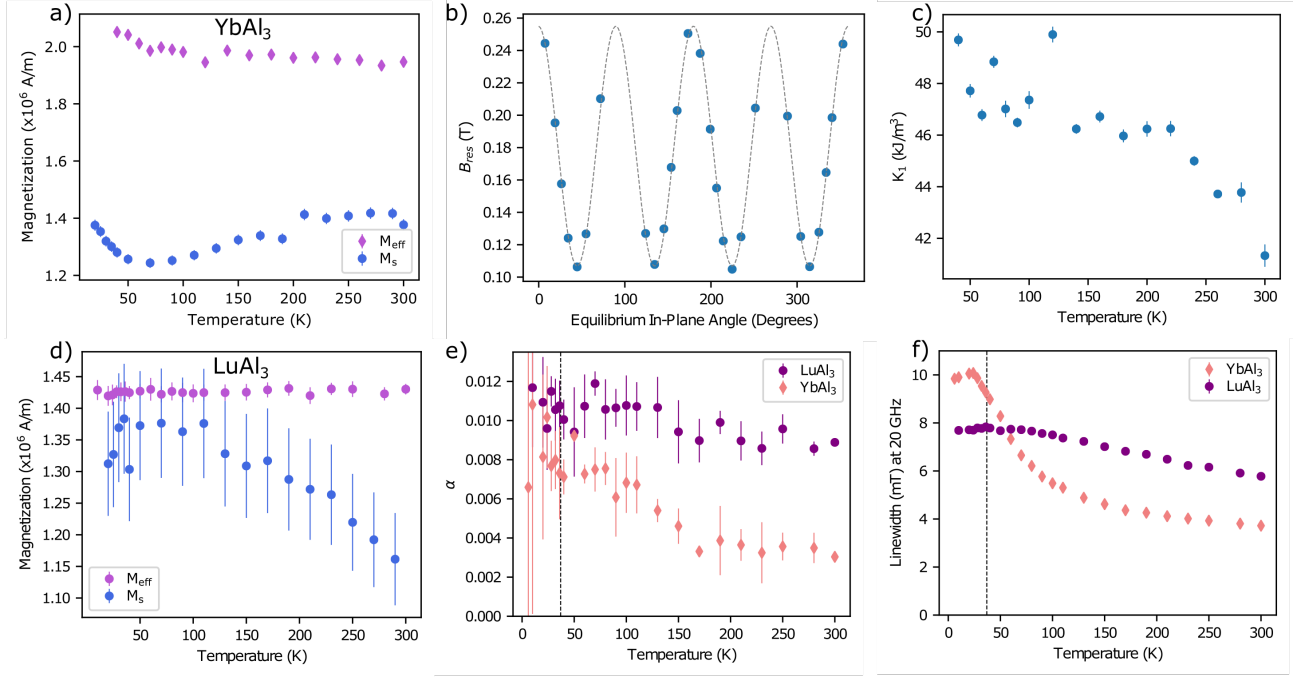

FIG. S2. Magnetic characterization of the Fe layer in both YbAl<sub>3</sub>/Fe (i.e., MgO (001)/Al 1.8 nm/LuAl<sub>3</sub> 5 nm/YbAl<sub>3</sub> 15 nm/Fe 6 nm/oxidized Al) and LuAl<sub>3</sub>/Fe (i.e., MgO (001)/Al 1.8 nm/LuAl<sub>3</sub> 15 nm/Fe 6 nm/oxidized Al). (a,d) Fe effective magnetization derived from the resonance condition in ST-FMR (Eq. (S2)) and the saturation magnetization extracted from vibrating sample magnetometry (purple diamonds and blue circles, respectively) of the (a) YbAl<sub>3</sub>/Fe and (d) LuAl<sub>3</sub>/Fe. (b) The ST-FMR resonant field as a function of in-plane magnetization angle for the YbAl<sub>3</sub>/Fe structure at 40 K (blue circles) with a fit to Eq. (S1) (dashed line). (c) Magnitude of the cubic anisotropy constant,  $K_1$ , extracted from the measurements in (b). (e) Gilbert damping parameter derived from a linear fit to the linewidth of the ST-FMR resonance curves vs. frequency from 18-20 GHz for YbAl<sub>3</sub>/Fe (orange diamonds) and LuAl<sub>3</sub>/Fe (purple circles), for magnetic fields applied along a magnetic easy axis of the Fe layer. (f) Linewidth at 20 GHz vs. temperature for YbAl<sub>3</sub>/Fe (orange diamonds) and LuAl<sub>3</sub>/Fe (purple circles). The vertical dashed line in (e) and (f) is at 37 K, the temperature below which Fermi liquid behavior is observed.

where  $B_{res}$  is the resonant field,  $\phi$  is the equilibrium direction of the magnetization for a given in-plane field angle with respect to the YbAl<sub>3</sub> [100] direction,  $\omega$  is the angular frequency of the driving current,  $\gamma$  is the electron gyromagnetic ratio,  $H_a$  is the anisotropy field defined as  $2K_1/M_s$  (where  $K_1$  is the first order cubic anisotropy constant), and  $M_{eff}$  is the effective magnetization including any contributions from an out of plane uniaxial anisotropy. Eq. S1 is the solution for  $B_{res}$  derived from resonance condition arising from an in-plane magnetized film with tetragonal magnetocrystalline anisotropy<sup>5</sup>:

$$f = \frac{\gamma}{2\pi} \sqrt{(B_{res} - 2H_a \cos(4\phi)) \left( B_{res} + \mu_0 M_{eff} + \frac{H_a}{2} (3 - \cos(4\phi)) \right)} \quad (S2)$$

The fit is recursively solved with the value of the equilibrium direction of the magnetization for each applied field angle recomputed at each step in the fitting process. This yields a  $K_1$  of 41 kJ/m<sup>3</sup> at 300 K which increases as the temperature is lowered to 50 kJ/m<sup>3</sup> at 40 K (Fig. S2c). As with  $M_s$ , these values for  $K_1$  are slightly smaller than the  $K_1$  found in crystalline Fe (48 kJ/m<sup>3</sup> at 300 K, 52 kJ/m<sup>3</sup> at 77 K)<sup>6</sup>.

From our fits to the resonant field vs. angle and at each temperature we also extract the effective magnetization shown as the purple diamonds in Figs. S2a) and d). We find an  $M_{eff}$  that increases with decreasing temperature and is non-trivially larger than  $M_s$  at a given temperature. This suggests that the small anti-parallel moment induced in the YbAl<sub>3</sub> layer also stabilizes the magnetization in plane.

Figs. S2e and f plot the Gilbert damping parameter,  $\alpha$ , vs. temperature.  $\alpha$  is extracted from the the frequency dependence of the linewidth,  $\Delta$  (determined from the fits to Eq.1 in the Methods section of the main text to our ST-FMR experiments), via a linear fit:

$$\Delta = \frac{\alpha\omega}{\gamma} + \Delta_{inhomo}, \quad (S3)$$

where  $\omega$  is the angular frequency of the applied RF current,  $\gamma$  is the electron gyromagnetic ratio, and  $\Delta_{\text{inhomo}}$  is the inhomogeneous component of the linewidth. Fitting to  $\Delta$  vs  $\omega$  for  $\frac{\omega}{2\pi}=18\text{-}20$  GHz yields the values of  $\alpha$  shown in Fig. S2e. We find the value of  $\Delta_{\text{inhomo}}$  to be negligible to within our error. The room temperature damping of  $\approx 0.003$  is consistent with the reported range of 0.002-0.004.<sup>7</sup> The peak in the linewidth vs temperature observed in Fig. S2f is characteristic of rare earth impurities in the ferromagnetic Fe layer,<sup>8,9</sup> and is likely a consequence of the direct growth of the Fe layer on the  $\text{YbAl}_3$ .

### C. Detailed description of the ST-FMR analysis

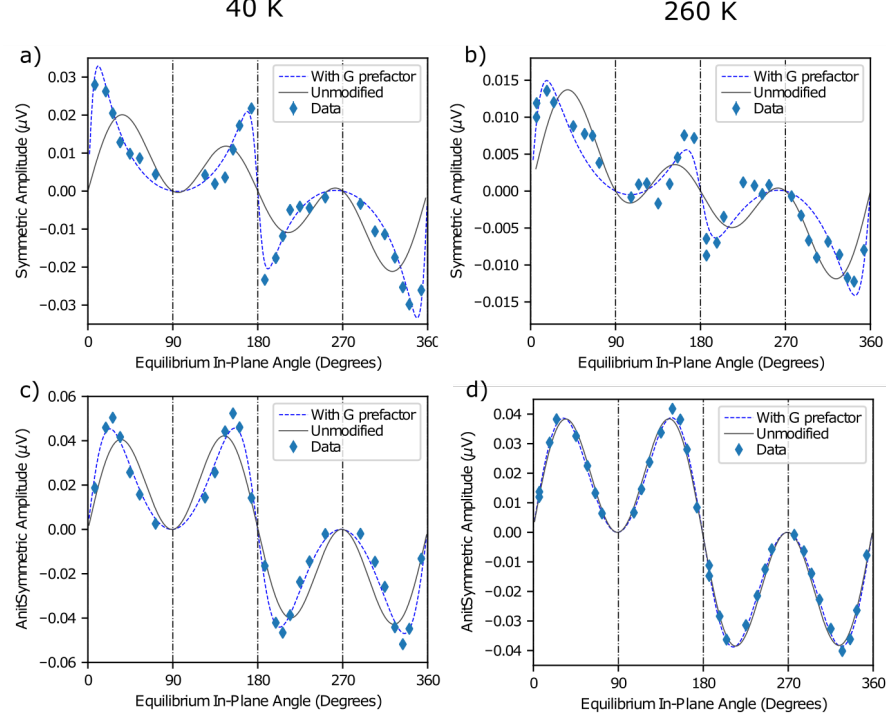

FIG. S3. (blue diamonds) Amplitudes of the (a,b) symmetric and (c,d) antisymmetric ST-FMR signals at  $f = 21$  GHz as a function of the angle of in-plane magnetization for the  $\text{YbAl}_3/\text{Fe}$  structure at (a,c) 40 K and (b,d) 260 K. The solid grey lines are fits to Eq. (S4) while the dashed blue lines are the fits to Eq. (S5) (i.e., the ST-FMR angular dependence with the phenomenological correction factor,  $G$ ). The vertical dashed lines correspond to the Fe layer magnetic hard axes (Fe [110]). The strength of the  $G$  term, and thus the degree to which the signal magnitudes grow near  $\phi = 0^\circ, 180^\circ$ , decreases at higher temperatures.

We perform two different measurements to fully analyze our ST-FMR data. In the first we apply a fixed frequency (21 GHz) and at each temperature measure the ST-FMR signal versus applied magnetic field magnitude for different angles of the applied field with respect to the current flow direction. From these scans, we extract the amplitude of the symmetric and antisymmetric Lorentzian components (as described in Methods) vs. the equilibrium in-plane magnetization angle,  $\phi$  (where  $\phi=0$  corresponds to the  $\text{YbAl}_3$  [100] direction, the Fe [110] direction, and the device current flow direction, see above). Representative angular dependences are shown in Fig. S3. The most general angular dependence allowed within a macrospin model for the symmetric and antisymmetric amplitudes of an ST-FMR resonance due to torque from a nonmagnetic material like  $\text{YbAl}_3$  has the functional form:

$$F(\phi) = \cos(\phi) \sin(\phi) (R \cos(\phi) + D \sin(\phi) + Z) \quad (\text{S4})$$

with  $R$ ,  $D$ , and  $Z$  potential components with Rashba-like, Dresselhaus-like, and out-of-plane uniaxial symmetry, respectively. The  $Z$  term for the antisymmetric component and the Dresselhaus-like terms for both components are not symmetry-allowed for  $\text{YbAl}_3/\text{Fe}$  samples, but we include them in fits as a check for artifacts. Even with this full angular dependence, we can observe deviations from the expected behavior in the regions just above and below  $\phi = 0^\circ$  and  $180^\circ$ , the two magnetic hard axes where the current-induced torques are strong (see Fig. S3a,b,d). Because these

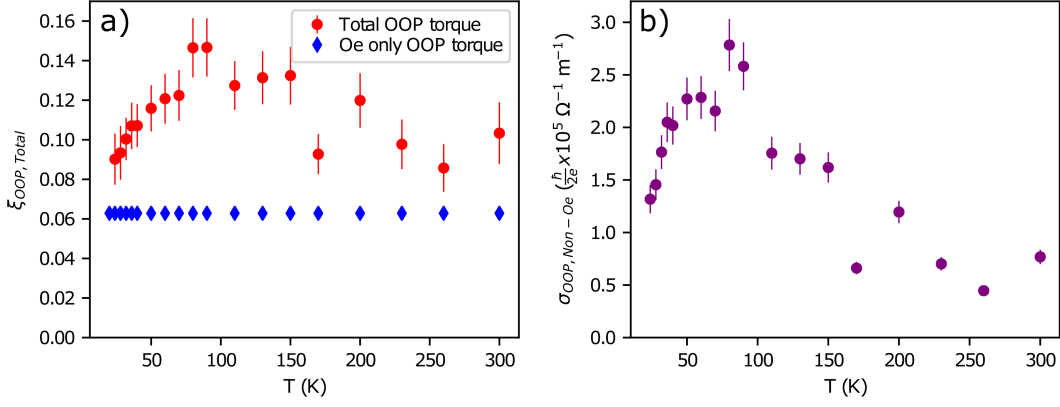

FIG. S4. (a) (red circles) Measured out-of-plane torque efficiency at  $f = 23$  GHz in the 1.8 nm Al/5 nm LuAl<sub>3</sub>/15 nm YbAl<sub>3</sub>/6 nm Fe/ oxidized Al heterostructure as a function of temperature. (blue diamonds) The calculated out-of-plane torque efficiency due to the Oersted field alone. (b) Effective spin-torque conductivity of the out-of-plane field-like spin-orbit torque determined from the difference between the measured changes and the expected Oersted contribution in (a).

deviations have an angular dependence incompatible with any component of current-induced torque in the macrospin model, we ascribe them to departures from macrospin dynamics. Iron has a relatively large value of  $M_{\text{eff}}$  and our apparatus is limited to frequencies  $f < 23$  GHz so as a consequence we are limited to measuring resonances with relatively small values of  $B_{\text{res}}$  for which the Fe magnetization may not remain fully saturated near the hard axes. To obtain quantitative results, we can determine the Rashba-like torques using only the ST-FMR amplitudes near the easy axes  $\phi = \pm 45^\circ, \pm 135^\circ$ . Alternately, we find that we obtain good fits to the full angular dependence by including a phenomenological angle-dependent scaling factor to account for an increased detection sensitivity near  $\phi = 0^\circ, 180^\circ$ :

$$F_{\text{corr}}(\phi) = \frac{\cos(\phi) \sin(\phi)}{1 + G \cos(2\phi)} (R \cos(\phi) + D \sin(\phi) + Z), \quad (\text{S5})$$

with  $G$  a fitting parameter. (Note that the added scaling factor does not change the values from  $F(\phi)$  at  $\phi = \pm 45^\circ, \pm 135^\circ$ , so fit values obtained are consistent with fixed-angle analyses at these angles.) Using this fitting function, as expected we observe large values only for the in-plane and out-of-plane torques with Rashba-like symmetries, with smaller contributions in some samples for the in-plane torque with out-of-plane uniaxial symmetry (at most 10 % of the in-plane torque with Rashba-like symmetry at low temperature where the in-plane torque is large). We suspect that the term with uniaxial symmetry is due to an out-of-plane Oersted field resulting from unequal current flow in the two arms of the ground-signal-ground contact geometry.

As described in the methods section, we use the change in resistance as a function of device power absorbed to determine the amount of RF current which reaches our device. This allows us to quantitatively determine the magnitude of the spin-orbit torques. Comparing the expected out-of-plane torque due the Oersted field with the measured out-of-plane calculated using the calibrated RF current reveals the presence of non-Oersted out-of-plane field-like torque as shown in Fig. S4a. The extracted spin torque conductivity for the non-Oersted out-of-plane field-like torque is shown in Fig. S4b. Due to this non-Oersted field-like torque, it is not accurate to apply the simple “S/A” analysis initially suggested in ref.<sup>10</sup>.

#### D. MOKE measurements of the low-temperature spin-orbit torque

MOKE measurements of the spin-orbit torque were performed on a home-built polar MOKE microscope using a Janis helium-flow cold-finger optical cryostat for temperature control. The measurements are modeled after ref.<sup>11</sup>. We apply a low frequency ( $< 6$  kHz) AC drive current to the device (shown in Fig. 3a) in the presence of an 80 mT external magnetic field parallel to the current flow direction. To ensure full saturation of the Fe layer, we use a bar fabricated along the Fe [100] direction easy axis (YbAl<sub>3</sub> [110]). Using a polar MOKE geometry so that we are sensitive only to the out-of-plane component of the magnetization and  $45^\circ$  linearly polarized light to minimize quadratic MOKE contributions ( $0^\circ$  corresponds to fully  $s$  polarized), we scan our laser spot across a  $60 \mu\text{m}$  wide by  $50 \mu\text{m}$  long device perpendicular to the current flow direction, and read out the spatial variation of the magnetization oscillation. Since the drive frequency ( $< 6$  kHz) is much lower than the natural frequency of the magnetization dynamics (several GHz),

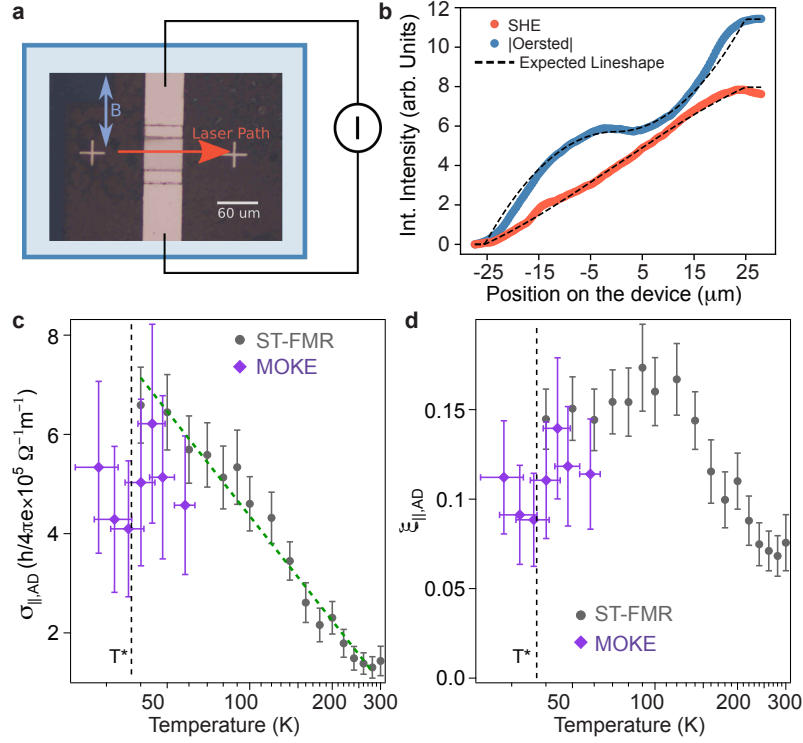

FIG. S5. MOKE measurements of current-induced torque in a 1.8 nm Al/5 nm LuAl<sub>3</sub>/15 nm YbAl<sub>3</sub>/6 nm Fe/ oxidized Al heterostructure. (a) MOKE experimental geometry showing the scan direction of the laser beam and the magnetic field direction. (b) Cumulative integrals as a function of position for the current-induced MOKE signal at 36 K. The “Oersted” curve is the integral of the absolute value of the signal that is an even function of the magnetization, while the “SHE” curve is the integral of the signal that is odd in the magnetization. The dashed lines are guides to the eye for the expected lineshapes. (c) Spin-orbit-torque conductivity and (d) spin-torque ratio derived from MOKE (purple diamonds), compared to the ST-FMR results for the same heterostructure.

we probe the quasi-static equilibrium shift of the magnetization due to the current-induced torques. This makes it possible to utilize the easily calculable form of the out-of-plane component of the Oersted field to calibrate the spatially uniform component of deflection due to the spin-orbit torque. We perform the same experiment at opposite fields to separate the Kerr response signals into odd (i.e. due to the effective field from the antidamping spin-orbit torque) and even (i.e. Oersted field) functions of magnetization. For the analysis, we numerically integrate both signals as a function of position (after taking the absolute value of the even signal first) and extract the spin-orbit torque from the ratio of the integral of the odd signal to the integral of the even signal. Figure 3b shows the cumulative integral of each signal with the simulated expected lineshapes.

The signal due to the in-plane spin-torques as a function of position across the device is given by the convolution of the beam shape with

$$V_d(B, x) = C \begin{cases} \xi_{||,AD} + \xi_{||,0}, & \text{for } B > 0; -\frac{w}{2} < x < \frac{w}{2} \\ -\xi_{||,AD} + \xi_{||,0}, & \text{for } B < 0; -\frac{w}{2} < x < \frac{w}{2} \\ 0, & \text{for } |x| > \frac{w}{2} \end{cases} \quad (\text{S6})$$

where  $V_d$  is the lockin voltage,  $B$  is the external magnetic field,  $x$  is the position of the scan with 0 centered in the middle of the device, and  $C = K \frac{\hbar J_c, \text{YbAl}_3}{2e M_s t_{\text{mag}} (B + M_{\text{eff}})}$ .  $K$  captures the Kerr constant and any other factors affecting the conversion of the optical response to a voltage signal from our split diode detector. The signal due to the Oersted

field generated due to current flowing within the device is given by the convolution of the beam shape with

$$V_s(B, x) = D \begin{cases} \ln \left( \frac{t^2 + (x - \frac{w}{2})^2}{t^2 + (x + \frac{w}{2})^2} \right), & \text{for } |B| > 0; -\frac{w}{2} < x < \frac{w}{2} \\ 0, & |x| > \frac{w}{2} \end{cases} \quad (\text{S7})$$

where  $D = K \frac{\mu_0 I_{total}}{2\pi w(B + M_{eff})}$  and  $\mu_0$  is the permeability of free space. Because we are measuring the out-of-plane component of the Oersted field, it is free from contamination due the non-Oersted out-of-plane spin-orbit torque that required careful consideration in the calibration of the ST-FMR signal. The signal due to  $\xi_{\parallel, AD}$  is odd in external field while the signals due to the Oersted field and  $\xi_{\parallel, 0}$  are even. Thus we can isolate the individual signals by adding and subtracting scans taken at two equal and opposite values of the external applied field ( $\pm 80$  mT in our experiment).

To extract values for the magnitude of the spin-orbit torques, we use that convolution is an area-preserving operation. The integral  $A_d$  as a function of position over the scan of Eq. S6 is

$$A_d \equiv C \xi_{\parallel, AD} w \quad (\text{S8})$$

and the integral of the absolute value of  $A_s$  over the scan of Eq. (S7) is

$$A_s \equiv Dw \ln(4) + C \xi_{\parallel, 0} w. \quad (\text{S9})$$

We take the absolute value before performing the spatial integral over  $A_s$  because Eq. (S7) is odd about  $x = 0$ . The integral of  $|A_s|$  therefore gives a convenient overall measure of the scale of the out-of-plane magnetic field, from which to calibrate the charge current within the nonmagnetic layers. We subtract out any offset due to  $\xi_{\parallel, 0}$  from the even signal before integration to get just the integral of the Oe signal  $A_{Oe} \equiv D \times w \ln(4)$ . Thus we can calculate

$$\xi_{\parallel, AD} = \frac{A_d}{A_{Oe}} \frac{\ln(4)D}{C} \quad (\text{S10})$$

$$= \frac{A_d}{A_{Oe}} \frac{e}{\hbar} \frac{\mu_0 M_s t_{mag} t_{total} \ln(4)}{X\pi} \quad (\text{S11})$$

where  $X$  is the fraction of the total current that flows through the YbAl<sub>3</sub> layer.

Figures S5c and d show a comparison between the in-plane antidamping spin-orbit torques measured using MOKE and ST-FMR on the same sample (a different sample than in Fig. 2 in the main text). The temperature stability of the optical cryostat limits our MOKE results to below 77 K, but in this range the MOKE results confirm very large values of antidamping spin-orbit torque conductivity, in agreement with the values determined by ST-FMR.

### E. Calculation of integrated spectral weight and background subtraction in YbAl<sub>3</sub> ARPES data

$E$ - $k$  spectral maps are obtained along the  $\Gamma$ -X direction using He I $\alpha$  (21.2 eV) photon energy that corresponds to a  $k_z$  value close to the bulk  $\Gamma$  point<sup>12</sup>. Momentum integrated energy distribution curves (EDC) were obtained from the spectral maps by integrating over a momentum region  $\pm(0.66 - 0.75)\pi/a$  as shown in Fig. 1b in the main text and also in Fig. S6b. The momentum region was chosen to minimize contribution from non Yb 4*f* derived bands, particularly the electron pocket near the  $\Gamma$  point. We used a Shirley background<sup>13</sup> to estimate the contribution of inelastically scattered electrons. Representative EDC plots before and after the background subtraction is shown in Figs. S6c-e. Integrated spectral weight plotted in Fig. 1e of the main text is obtained by calculating the area under the curve over a binding energy region between -0.05 eV and 0.2 eV after background subtraction. Following the above procedure we obtain an enhancement ratio for the integrated spectral weight as  $\frac{I(37K)}{I(255K)} = 2.2$ . Considering the intensity of the Kondo resonance (peak heights) in the EDC plots we obtain a ratio of 3.8. The obtained enhancement factor depends on the chosen binding energy range over which the spectral weight integration is performed and also on the details of the background subtraction and is found to vary between  $\frac{I(37K)}{I(255K)} \approx 2$  and 4. Temperature dependent scaling behavior as described in the main text and saturation behavior at  $T^*$  are found to be robust both to the choice of binding energy integration window and background subtraction procedure.



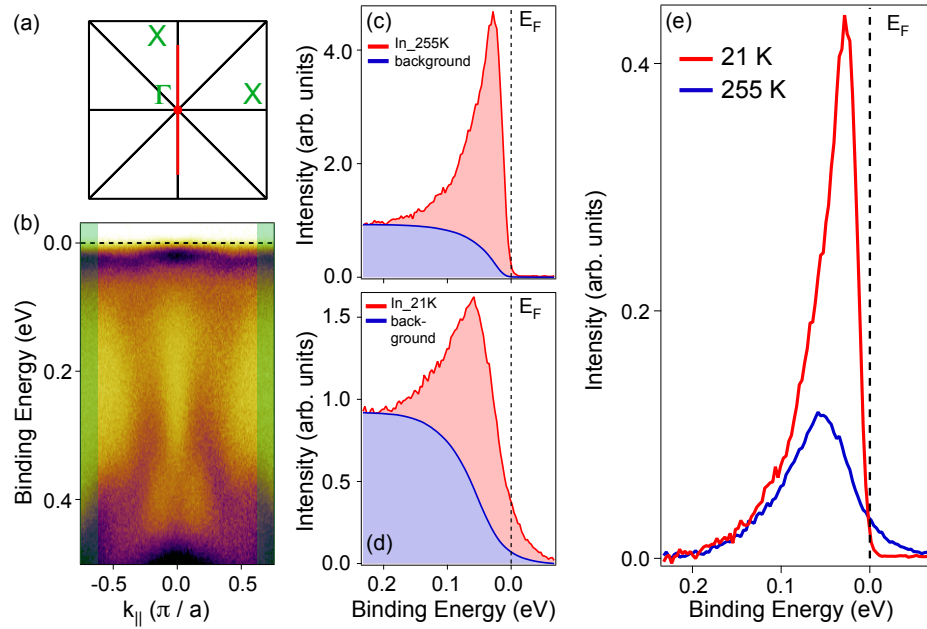

FIG. S6. (a) Surface Brillouin zone of YbAl<sub>3</sub> showing high symmetry points. (b)  $E$ - $k$  spectral map taken at 31 K corresponding to the ARPES cut (red line) shown in (a). Energy distribution curves taken at (c) 21 K and (d) 255 K integrated over the momentum region highlighted in green in (b). A Shirley background that takes into account contributions from inelastically scattered electrons is shown in blue. (e) Background-subtracted energy distribution curves at 21 K and 255 K.

- 
- [1] Chatterjee, S. *et al.* Epitaxial growth and electronic properties of mixed valence YbAl<sub>3</sub> thin films. *J. Appl. Phys.* **120**, 035105 (2016).
  - [2] Taylor, G., Isin, A. & Coleman, R. Resistivity of iron as a function of temperature and magnetization. *Phys. Rev.* **165**, 621 (1968).
  - [3] Hiess, A., Boucherle, J., Givord, F. & Canfield, P. Magnetic susceptibility and magnetization measurements of an YbAl<sub>3</sub> single crystal for groundstate investigations. *J. Alloys Compd.* **224**, 33–35 (1995).
  - [4] Crangle, J. & Goodman, G. The magnetization of pure iron and nickel. *Proc. R. Soc. London, Ser. A* **321**, 477–491 (1971).
  - [5] Farle, M. Ferromagnetic resonance of ultrathin metallic layers. *Rep. Prog. Phys.* **61**, 755 (1998).
  - [6] Graham Jr, C. Magnetocrystalline anisotropy constants of iron at room temperature and below. *Phys. Rev.* **112**, 1117 (1958).
  - [7] Stearns, M. B. 1.1.2.10 g factors and ferromagnetic resonance properties: Datasheet from Landolt-Börnstein - Group III Condensed Matter · Volume 19A: “3d, 4d and 5d Elements, Alloys and Compounds” in SpringerMaterials ([https://doi.org/10.1007/10311893\\_13](https://doi.org/10.1007/10311893_13)). URL [https://materials.springer.com/lb/docs/sm\\_lbs\\_978-3-540-39667-3\\_13](https://materials.springer.com/lb/docs/sm_lbs_978-3-540-39667-3_13).
  - [8] Bailey, W., Kabos, P., Mancoff, F. & Russek, S. Control of magnetization dynamics in ni/sub 81/fe/sub 19/ thin films through the use of rare-earth dopants. *IEEE Trans. Magn.* **37**, 1749–1754 (2001).
  - [9] Seiden, P. E. Ferrimagnetic resonance relaxation in rare-earth iron garnets. *Phys. Rev.* **133**, A728–A736 (1964).
  - [10] Liu, L., Moriyama, T., Ralph, D. C. & Buhrman, R. A. Spin-torque ferromagnetic resonance induced by the spin Hall effect. *Phys. Rev. Lett.* **106**, 036601 (2011).
  - [11] Fan, X. *et al.* Quantifying interface and bulk contributions to spin-orbit torque in magnetic bilayers. *Nat. Comm.* **5**, 3042 (2014).
  - [12] Chatterjee, S. *et al.* Lifshitz transition from valence fluctuations in YbAl<sub>3</sub>. *Nat. Commun.* **8**, 852 (2017).
  - [13] Shirley, D. A. High-resolution x-ray photoemission spectrum of the valence bands of gold. *Phys. Rev. B* **5**, 4709 (1972).
